# Supplementary material for: Geometry of Deep Generative Models for Disentangled Representations
Source: arXiv:1902.06964 source file (2019-02-19)
Supplement: Supplementary file 1 [file additional_5classes.tex]

% this is clustering for 5 classes
\documentclass[a4paper]{article}

\usepackage[english]{babel}
\usepackage[utf8]{inputenc}
\usepackage{amsmath}
\usepackage{graphicx}
\usepackage[colorinlistoftodos]{todonotes}

\title{Additional Results}

\author{Your names and group number}

\date{\today}

\begin{document}
\begin{center}
\begin{tabular}{|c|c|c|c|} 
 \hline
 Model & Szabo \emph{et al} & Mathieu \emph{et al} & Jha \emph{et al} \\\hline
 Euclidean F Score & 92.68 & 96.32 & 95.14 \\\hline 
 Riemannian F Score & 96.84 & 98.92 & 97.44 \\ \hline
 \end{tabular}
 \end{center}

 \end{document}
