# Supplementary material for: Geometry of Deep Generative Models for Disentangled Representations
Source: arXiv:1902.06964 source file (2019-02-19)
Supplement: Supplementary file 2 [file additional_chairs.tex]

% chairs
\documentclass[a4paper]{article}

\usepackage[english]{babel}
\usepackage[utf8]{inputenc}
\usepackage{amsmath}
\usepackage{graphicx}
\usepackage[colorinlistoftodos]{todonotes}

\title{Additional Results}

\author{Your names and group number}

\date{\today}

\begin{document}
\begin{center}
\begin{tabular}{|c|c|c|c|} 
 \hline
 Model & Szabo \emph{et al} & Mathieu \emph{et al} & Jha \emph{et al} \\\hline
 Euclidean F Score & 91.16 & 94.33 & 94.24 \\\hline 
 Riemannian F Score & 95.22 & 96.34 & 96.44 \\ \hline
 \end{tabular}
 \end{center}
 
 \begin{center}
\begin{tabular}{|c|c|c|c|} 
 \hline
 Model & VAE & Szabo \emph{et al} & Mathieu \emph{et al} & Jha \emph{et al} \\\hline
 C values on 3D Chairs & 0.162 & 0.262 & 0.311 & 0.315 \\\hline 
 \end{tabular}
 \end{center}
 
 \begin{center}
\begin{tabular}{|c|c|c|c|} 
 \hline
 Model & Szabo \emph{et al} & Mathieu \emph{et al} & Jha \emph{et al} \\\hline
 Normalized Margin on 3D Chairs & 0.492 & 0.529 & 0.525 \\\hline 
 \end{tabular}
 \end{center}
 
 \begin{center}
\begin{tabular}{|c|c|c|c|} 
 \hline
 Model & Szabo \emph{et al} & Mathieu \emph{et al} & Jha \emph{et al} \\\hline
 Euclidean Distance & 0.158 & 0.160 & 0.156 \\\hline 
 Riemannian Distance & 0.344 & 0.376 & 0.365 \\\hline 
 \end{tabular}
 \end{center}
 
 \begin{center}
\begin{tabular}{|c|c|c|c|} 
 \hline
 Model & VAE & Szabo \emph{et al} & Mathieu \emph{et al} & Jha \emph{et al} \\\hline
 Curvature on 3D Chairs & 23.45 & 36.77 & 35.86 & 36.50 \\\hline 
 \end{tabular}
 \end{center}

 \end{document}
